# Supplementary material for: Quantum noise spectroscopy of superconducting dynamics in a cuprate thin film
Source: arXiv:2502.04439 source file (2026-10-27)
Supplement: Supplementary file 1 [file supp.pdf]

# Supplementary Information: Quantum noise spectroscopy of superconducting dynamics in thin film $\text{Bi}_2\text{Sr}_2\text{CaCu}_2\text{O}_{8+\delta}$

Zhongyuan Liu,<sup>1,\*</sup> Ruotian Gong,<sup>1,\*</sup> Jaewon Kim,<sup>2,\*</sup> Oriana K. Diessel,<sup>3,4,\*</sup> Qiaozhi Xu,<sup>1</sup> Zackary Reh fuss,<sup>1</sup>  
Xinyi Du,<sup>1</sup> Guanghui He,<sup>1</sup> Abhishek Singh,<sup>5</sup> Yun Suk Eo,<sup>5</sup> Erik A. Henriksen,<sup>1,6</sup> G. D. Gu,<sup>7</sup>  
Norman Y. Yao,<sup>4</sup> Francisco Machado,<sup>3,4</sup> Sheng Ran,<sup>1,6</sup> Shubhayu Chatterjee,<sup>8,†</sup> Chong Zu<sup>1,6,‡</sup>

<sup>1</sup>Department of Physics, Washington University, St. Louis, Missouri 63130, USA

<sup>2</sup>Department of Physics, University of California, Berkeley, California 94720, USA

<sup>3</sup>ITAMP, Center for Astrophysics, Harvard & Smithsonian, Cambridge, Massachusetts 02138, USA

<sup>4</sup>Department of Physics, Harvard University, Cambridge, Massachusetts 02138, USA

<sup>5</sup>Department of Physics and Astronomy, Texas Tech University, Lubbock, Texas 79409, USA

<sup>6</sup>Institute of Materials Science and Engineering, Washington University, St. Louis, Missouri 63130, USA

<sup>7</sup>Condensed Matter Physics and Materials Science Department,  
Brookhaven National Laboratory, Upton, New York 11973, USA

<sup>8</sup>Department of Physics, Carnegie Mellon University, Pittsburgh, Pennsylvania 15213, USA

\*These authors contribute equally to this work

<sup>†</sup>To whom correspondence should be addressed; E-mail: shubhayuchatterjee@cmu.edu

<sup>‡</sup>To whom correspondence should be addressed; E-mail: zu@wustl.edu

(Dated: February 27, 2025)

## CONTENTS

|                                                                           |   |
|---------------------------------------------------------------------------|---|
| I. Nitrogen-vacancy center                                                | 1 |
| I.1. Optically detected magnetic resonance                                | 2 |
| I.2. NV ensemble spin relaxation                                          | 2 |
| I.2.1. Consistency between different methods of extracting the decay rate | 3 |
| I.3. NV ensemble spin decoherence                                         | 4 |
| II. Experimental details                                                  | 4 |
| II.1. Setup apparatus                                                     | 4 |
| II.2. Creation of NV centers                                              | 4 |
| II.3. BSCCO sample preparation                                            | 5 |
| II.4. Off-axis $T_1$ relaxometry                                          | 5 |
| II.5. The pinned superconducting vortex                                   | 6 |
| References                                                                | 7 |

## I. NITROGEN-VACANCY CENTER

The nitrogen-vacancy (NV) center in diamond is a color defect in diamond crystals, consisting of a nitrogen atom replacing a carbon atom adjacent to a vacancy in the carbon lattice [1]. The electronic ground state of a negatively charged NV center forms a spin-1 triplet state. In the absence of external disturbances, the  $|m_s = 0\rangle$  sublevel is separated from the degenerate  $|m_s = \pm 1\rangle$  sublevels by a temperature-dependent zero-field splitting  $D_{\text{gs}} = 2.87$  GHz, along the quantization axis  $\hat{z}$  in N-V direction.

In the presence of a magnetic field, the axial component  $B_z$  lifts the degeneracy between  $|m_s = \pm 1\rangle$  states with a Zeeman splitting  $2\gamma_e B_z$ , where  $\gamma_e = 2.8$  MHz/G is the electronic spin gyromagnetic ratio. Additionally, the local electric charges around NV centers will couple to the system [2], represented by the Hamiltonian:

$$\mathcal{H}_E = \Pi_z S_z^2 + \Pi_x (S_y^2 - S_x^2) + \Pi_y (S_x S_y + S_y S_x), \quad (\text{S1})$$

where  $\{S_x, S_y, S_z\}$  are the spin-1 operators,  $\Pi_{\{x,y\}} = d_{\perp} E_{\{x,y\}}$  and  $\Pi_z = d_{\parallel} E_z$  characterize the coupling strength to the electric field  $\vec{E}$  with susceptibilities  $\{d_{\perp}, d_{\parallel}\} = \{17, 0.35\}$  Hz · cm/V [3]. Given that  $d_{\perp} \gg d_{\parallel}$ , the axial term  $\Pi_z$

can be neglected. Meanwhile, the transverse terms only couple to the  $|m_s = \pm 1\rangle$  states, producing new eigenstates:

$$|+\rangle = \frac{1}{\sqrt{2}} (|m_s = +1\rangle + e^{i\theta}|m_s = -1\rangle) \quad (\text{S2})$$

$$|-\rangle = \frac{1}{\sqrt{2}} (|m_s = +1\rangle - e^{i\theta}|m_s = -1\rangle) \quad (\text{S3})$$

where  $\theta = \arctan(\Pi_y/\Pi_x)$  represents the transverse orientation of electric field. This interaction introduces an energy splitting of  $2\Pi_{\perp} = 2\sqrt{\Pi_x^2 + \Pi_y^2}$ . As a result, the local-charge-induced splitting combines in quadrature with the Zeeman splitting, leading to a total splitting of  $\Delta = \sqrt{(2\Pi_{\perp})^2 + (2\gamma_e B_z)^2}$  shown in the ODMR spectrum.

### I.1. Optically detected magnetic resonance

In this work, we perform a continuous-wave optically detected magnetic resonance (ODMR) spectroscopy to probe transitions between different spin-states of the NV. During the measurement, both the laser and microwave driving fields remain on, while the frequency of the microwave field is swept. The NV spins are polarized into their initial state,  $|m_s = 0\rangle$ . When the microwave is off-resonant, the NV centers remain in  $|m_s = 0\rangle$ . As the microwave is swept onto resonance with one of the spin transitions, the spin population is driven into  $|m_s = \pm 1\rangle$ , resulting in a decrease of NV fluorescence.

Depending on the orientation of the external magnetic field relative to the NV axis, the axial magnetic field  $B_z$  varies according to the crystallographic directions of the diamond bonds. This variation leads to four subgroups of NV centers. Throughout our experiment, the external magnetic field is along the out-of-plane direction of the [111]-cut diamond, aligning with one NV group. In this configuration, the ODMR spectrum exhibits four distinct resonant peaks, as shown in the bottom panel of Fig. 2(a) in the main text. The NV group aligned with the field experiences the largest magnetic field projection, giving rise to the outer two resonances with a splitting  $\Delta$ . Meanwhile, the remaining NV groups in the other three directions are degenerate, contributing to the inner peaks.

### I.2. NV ensemble spin relaxation

To characterize the spin relaxation of NV ensemble, we perform a differential sequence to measure the lifetime of  $|m_s = 0\rangle$  state, while mitigating the NV charge dynamics effect under laser pumping [4], see Figure S1(a). To be specific, we first let NV charge dynamics reach equilibration by waiting for 100  $\mu\text{s}$  without laser illumination (I). Next, a 15  $\mu\text{s}$  laser pulse is applied to initialize the NV centers to  $|m_s = 0\rangle$  state (II). A reference readout  $S_R$  is taken at the end of the pulse. After the polarization, we pause for a variable time period  $\tau$  for spin relaxation (III), then turn on the laser to detect the spin population of bright state  $|m_s = 0\rangle$  as  $S_B(\tau)$  (IV). Finally, we repeat the I-IV procedures but with a  $\pi$ -pulse at the end of time  $\tau$  to swap the population from dark state  $|m_s = \pm 1\rangle$ , recorded as  $S_D(\tau)$ , to  $|m_s = 0\rangle$ . As a result, the relaxation time  $T_1$  is extracted by fitting the fluorescence contrast to a stretched exponential decay

$$C(\tau) = \frac{S_B(\tau) - S_D(\tau)}{S_R} \propto e^{-\left(\frac{\tau}{T_1}\right)^{\alpha_1}}, \quad (\text{S4})$$

where the stretched power  $\alpha_1 = 1/2$  according to a pioneering study [4].

To quantitatively analyze the relaxation rate induced from the fluctuation noise, we treat the overall decay as a combination of an intrinsic decay and the noise-related decay,

$$C(\tau) \sim e^{-\sqrt{\tau/T_1}} = e^{-\sqrt{\Gamma_1^{\text{total}} \tau}} = e^{-\sqrt{\Gamma_1^{\text{int}} \tau}} \cdot e^{-\sqrt{\Gamma_1^{\text{noise}} \tau}}. \quad (\text{S5})$$

Then the decay rate  $\Gamma_1^{\text{noise}}$ , shorten as  $\Gamma_1$  in the main text, can be written as

$$\Gamma_1 = \left( \sqrt{\Gamma_1^{\text{total}}} - \sqrt{\Gamma_1^{\text{int}}} \right)^2, \quad (\text{S6})$$

with  $\Gamma_1^{\text{total}}$ ,  $\Gamma_1^{\text{int}}$  respectively extracted from the measurements at NV centers under and away BSCCO flake.

For  $T_1$ -based noise spectroscopy, the spin depolarization dynamics are determined by the magnetic noise spectrum

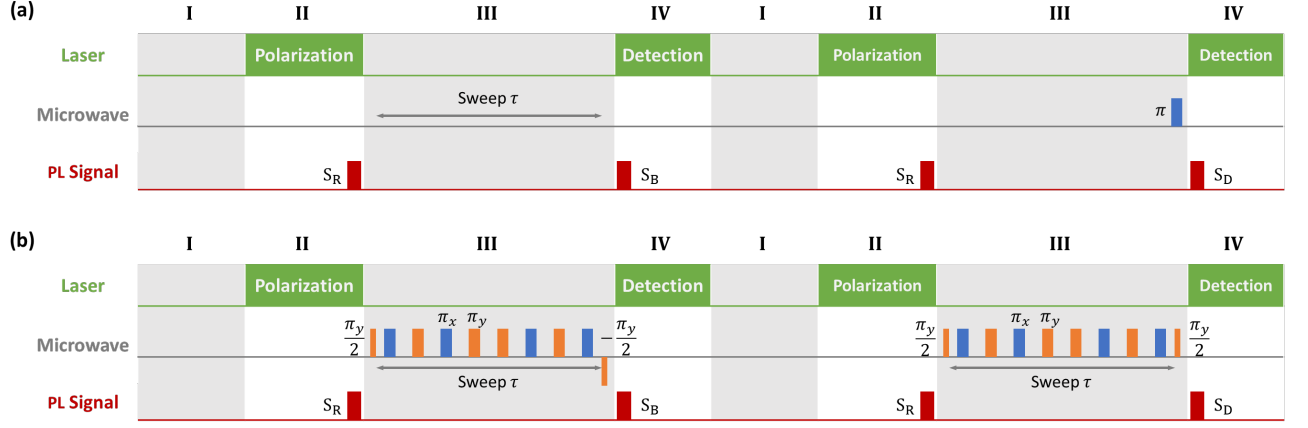

FIG. S1. **Differential pulse sequences.** (a) Schematic of  $T_1$  sequence. (b) Schematic of XY-8 sequence.

at the NV resonance frequencies  $\omega \simeq D_{gs} \pm \Delta/2$ , leading to a sharp frequency filter function  $W_\tau(\omega)$  peaked in the GHz range.

### I.2.1. Consistency between different methods of extracting the decay rate

The methodology used to extract the BSCCO-induced decay and decoherence rates, denoted as  $\Gamma_1$  and  $\Gamma_2$  in the main text respectively, are outlined in Sections I.2 and I.3. In this section, drawing inspiration from a previous study [5], we introduce an alternative method to validate the reliability of our findings.

For each temperature, we measure the fluorescence contrast as a function of the time interval  $\tau$ ,  $C(\tau)$ , for NV centers both under and away from BSCCO, and normalize the values to 1. Taking the fluorescence measured at NV centers away from BSCCO as a reference,  $C_{\text{ref}}(\tau)$ , we define a normalized decay:

$$C_{\text{norm}}(\tau) = \frac{C(\tau)}{C_{\text{ref}}(\tau)} = e^{-\sqrt{\Gamma_1^*} \tau}, \quad (\text{S7})$$

where  $\Gamma_1^*$  is the noise-induced decay rate. An example of this is shown in Fig. S2(a). By fitting  $C_{\text{norm}}(\tau)$  to a stretched exponential decay with a power 1/2, we extract the temperature dependence of the BSCCO-induced decay rate  $\Gamma_1^*(T)$ , which is summarized as Method 2 in Fig. S2(b). Compared to  $\Gamma_1(T)$  extracted using the Method 1 in Section I.2,  $\Gamma_1^*(T)$  has a same asymmetry profile, with nearly identical peak amplitude and position. This consistency underscores the robustness of our results.

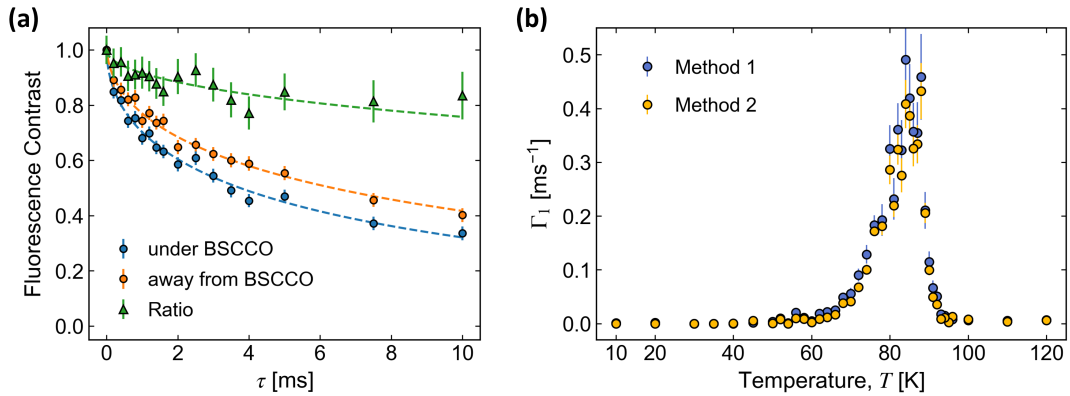

FIG. S2. **Comparing different methods.** (a) The relaxation decays of NV centers under (blue) and away (orange) from BSCCO at  $T = 100$  K and  $H = 40$  G. The data in green color is calculated via dividing the blue data with the orange data. All data are fitted with an exponential decay with a stretched power 1/2. (b) The temperature dependence of the BSCCO-induced relaxation rate  $\Gamma_1$  extracted using two methods.

### I.3. NV ensemble spin decoherence

We apply a dynamical decoupling pulse sequence, XY-8 [6], to probe the spin decoherence properties of NV ensemble, see Figure S1(b). Comparing to the commonly used Spin Echo pulse sequence, instead of a single refocusing  $\pi$ -pulse in the middle, XY-8 employs a series of  $\pi$ -pulses with alternating phases. As a result, XY-8 further suppresses the local spin noise and is self-compensating for pulse errors.

Similar to spin relaxation, the spin coherence time  $T_2$  follows a stretched exponential decay profile

$$C(\tau) \propto e^{-\left(\frac{\tau}{T_2}\right)^{\alpha_2}}, \quad (\text{S8})$$

with a stretched power  $\alpha_2 = 3/2$  for NV ensemble [7].

The decoherence rate induced from the fluctuation noise,  $\Gamma_2$ , takes the form

$$\Gamma_2 = \left( (\Gamma_2^{\text{total}})^{\frac{3}{2}} - (\Gamma_2^{\text{int}})^{\frac{3}{2}} \right)^{\frac{2}{3}}, \quad (\text{S9})$$

where  $\Gamma_2^{\text{total}}$ ,  $\Gamma_2^{\text{int}}$  extracted from NV centers under and away from the BSCCO flake. To ensure the non-negative value inside the parentheses, any negative results are capped at zero.

In contrast to  $T_1$ -based noise spectroscopy, the filter function of  $T_2$ -based noise spectroscopy can be tailored by the time interval  $\tau$ , see supplementary material in [8]:

$$W_{\tau}^{(\text{XY8})}(\omega) \sim \frac{\sin^2 \frac{\omega\tau}{2}}{\omega^2} \cdot \frac{\sin^4 \frac{\omega\tau}{32}}{\cos^2 \frac{\omega\tau}{16}}. \quad (\text{S10})$$

It peaks at  $\omega \simeq 8\pi/\tau$ , with width  $\sim \pi/\tau$ . In this work, the time  $\tau$  is swept up to  $\sim 10 \mu\text{s}$ , enabling a noise spectroscopy that is sensitive to the MHz range.

## II. EXPERIMENTAL DETAILS

### II.1. Setup apparatus

We perform NV measurements in a commercial low-vibration closed-cycle cryostat (Fournine Design SK200), equipped with optical access facilitated by a custom-built confocal scanning microscope. The initialization and detection of NV center spins are driven by a laser light with wavelength  $\lambda = 532 \text{ nm}$  (Millennia eV High Power CW DPSS Laser). The laser is modulated by an acousto-optic modulator (AOM, G&H AOMO 3110-120) in a double-pass configuration to achieve an on/off ratio exceeding  $10^5 : 1$ . The lateral scanning is performed using a X-Y galvanometer (Thorlabs GVS212), in combination with a 4f-telescope setup. A piezo objective scanner (Physik Instrumente P-721.SL2) controls the vertical position with  $100 \mu\text{m}$  travel range. The laser beam is focused onto the sample by an objective lens (Mitutoyo Plan Apo 20x/0.42 NA) mounted on the piezo scanner, achieving a diffraction-limited spot size with a diameter less than  $1 \mu\text{m}$ . The NV fluorescence is collected by the same objective, separated from the laser beam via a dichroic mirror and filtered through a long-pass filter before being detected by a single photon counting module (Excelitas SPCM-AQRH-63-FC). The signal is processed by a data acquisition device (National Instruments USB-6343). The microwave driving field for NV spin control is generated from a signal generator (Stanford Research Systems SG384), amplified by a high-power amplifier (Mini-Circuits ZHL-15W-422-S+) and gated through a switch (Minicircuits ZASWA-2-50DRA+) to prevent any potential leakage. All equipment are synchronized via a programmable multi-channel pulse generator (SpinCore PulseBlasterESR-PRO 500) with 2 ns temporal resolution.

The cryostat is cooled down to base temperature below 4 K by a closed-cycle helium compressors (Sumitomo F-40L). A cryogenic temperature controller (LakeShore Model 336) and a sample temperature sensor with integrated heaters are employed to maintain samples at desired temperature in range from 4 K to 350 K.

### II.2. Creation of NV centers

In this work, we use a double-side polished single crystal type-Ib diamond plate in shape of  $2.5 \text{ mm} \times 2.5 \text{ mm} \times 0.3 \text{ mm}$  with [111]-cut surfaces (Sumitomo). The diamond is synthesized through a high-pressure high-temperature (HPHT) process, with  $[\text{N}] < 200 \text{ ppm}$  [9]. We employ  $^{12}\text{C}^+$  ion implantation (CuttingEdge Ions, LLC) at 12 keV energy with a dosage of  $2.25 \times 10^{11} \text{ cm}^{-2}$  and 30 keV energy with a dosage of  $6.75 \times 10^{11} \text{ cm}^{-2}$  sequentially. We

perform a detailed calculation with full damage cascades using Stopping and Range of Ions in Matter (SRIM) [10] to obtain the total created NV defect density distribution. As a result, a  $\sim 50$  nm layer of vacancies is generated below the plate surface, see Fig. S3. After implantation, the diamond is placed in vacuum ( $< 10^{-6}$  mbar) and annealed in a home-built furnace with a recipe same to previous work [11]: 12 hours ramp to  $400^\circ\text{C}$ , dwell for 8 hours, 12 hours ramp to  $800^\circ\text{C}$ , dwell for 8 hours, 12 hours ramp to  $1050^\circ\text{C}$ , dwell for 2 hours. The NV concentration after the annealing process is estimated to be around 1 ppm.

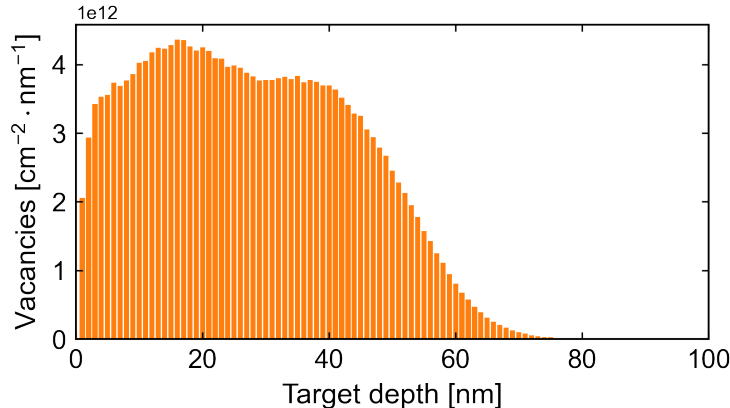

FIG. S3. The vacancy density as a function of the depth below surface, calculated using Stopping and Range of Ions in Matter (SRIM). The vacancies are concentrated in the first  $\sim 50$  nm layer beneath the diamond surface.

### II.3. BSCCO sample preparation

The  $\text{Bi}_2\text{Sr}_2\text{CaCu}_2\text{O}_{8+\delta}$  (BSCCO, Bi-2212) single crystals used in this work are grown by the traveling floating zone technique [12]. We exfoliate BSCCO flakes using Scotch tape and transfer them directly onto the diamond surface. Due to the air-sensitivity of BSCCO, we immediately enclose the sample in a vacuum environment within the cryostat. To estimate the thickness of the target flake, we exfoliate additional flakes separately and identify several with similar optical contrast to the target. We then measure their thickness using atomic force microscopy. The measured thicknesses range from  $188 \pm 5$  nm to  $300 \pm 10$  nm, leading us to estimate that the target flake is approximately 200 nm thick. The total air exposure time is kept under an hour, and given the flake's thickness, this brief exposure is not expected to significantly impact its superconducting properties.

### II.4. Off-axis $T_1$ relaxometry

Relaxation-based ( $T_1$ ) noise spectroscopy of NV centers is primarily sensitive to fluctuating components of the magnetic field perpendicular to the NV quantization axis, which, in our case, corresponds to the in-plane direction, i.e.  $B_x(t)$  and  $B_y(t)$ . To further probe the other components of the magnetic noise tensor, corresponding to a time-varying  $B_z(t)$  arising from current fluctuations, we also perform the relaxation spectroscopy on the off-axis NV centers — specifically, the NV groups in the other three crystal orientations, as illustrated in Fig. 1(b) in the main text. In our setup geometry, the  $[111]$  NV group is aligned along the out-of-plane direction, while the other three groups ( $[\bar{1}1\bar{1}]$ ,  $[\bar{1}\bar{1}1]$ ,  $[1\bar{1}\bar{1}]$ ) are mainly in-plane, forming an angle  $\theta = \arcsin(\frac{1}{3})$  with the surface. Consequently, the  $[111]$  group serves as a sensor for in-plane magnetic field fluctuations, whereas the non- $[111]$  groups can also detect the out-of-plane signals.

In the absence of magnetic field, all four NV groups are degenerate, making the sensor equally responsive to signals in all directions. When a bias field is applied along the out-of-plane direction, the  $[111]$  group exhibits greater splitting in the ODMR spectrum due to its larger field projection, as shown in Fig. 2(a) bottom panel in the main text. By selecting the appropriate resonance frequency, we can independently measure the relaxation timescales of either  $[111]$  or non- $[111]$  NV groups. Figure S4 shows the temperature dependence of the BSCCO-induced relaxation rate  $\Gamma_1$  for both  $[111]$  NV group and non- $[111]$  NV groups under an external magnetic field  $H = 40$  G. Compared to the NVs aligned with the field, the peak position of  $\Gamma_1(T)$  for the off-axis NVs remains largely unchanged, i.e., the peak in  $\Gamma_1(T)$  occurs at a higher temperature than the  $\Gamma_2(T)$  peak [see Fig. 4(b) in the main text]. This observation is

consistent with the expectation that current fluctuations in the sample can contribute to time-varying magnetic fields in all three directions  $x, y, z$ , and adds further credence to the interpretation of the peak in  $\Gamma_1(T)$  as arising from enhanced current fluctuations near criticality.

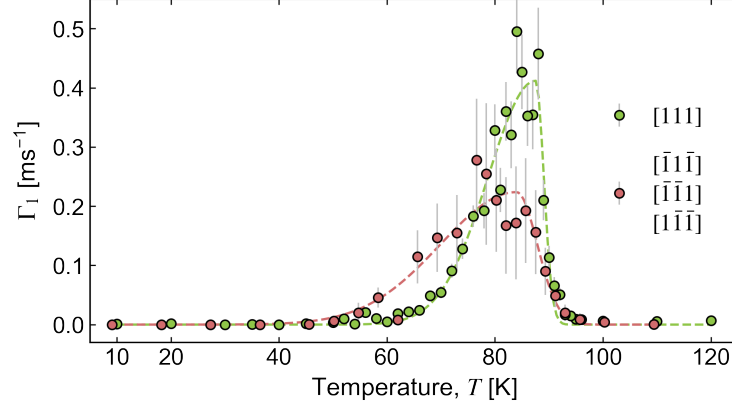

FIG. S4. **Off-axis  $T_1$  relaxometry.** The  $\Gamma_1$  as a function of temperature for [111] NV group (green) and non-[111] NV groups (red) under a bias field  $H = 40$  G.

### II.5. The pinned superconducting vortex

In this subsection, we provide additional details on the defect-trapped vortex discussed in Fig. 4(d) in the main text. By performing ODMR measurements on NV centers in the region highlighted by a rectangle in the left panel of Fig. S5, we obtain a two-dimensional local magnetic field map near the edge of the BSCCO flake under an applied bias magnetic field of  $H = 40$  G. As shown in the bottom panel of Fig. S5, above the critical temperature ( $T = 110$  K), the local magnetic field  $B_z$  is nearly uniform across the entire area. However, at  $T = 45$  K, well below the critical temperature,  $B_z$  is enhanced at the edge of the BSCCO flake, and suppressed beneath it. More importantly, a vortex appears in the area under the flake. We note the position of the vortex remains consistent across multiple temperature sweeps, suggesting it may be pinned by a local defect.

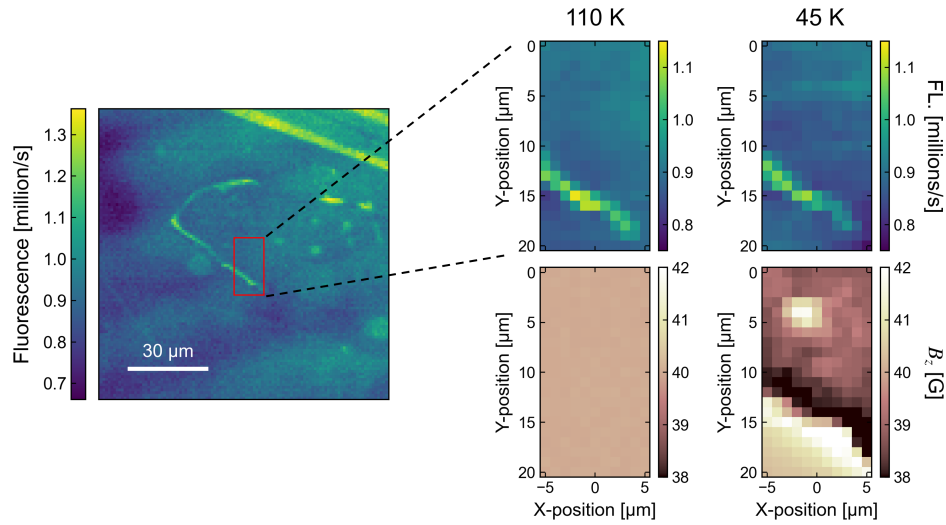

FIG. S5. **Image of a pinned superconducting vortex.** Left: a fluorescence scan image of the BSCCO flake on the diamond surface. Right top: zoom-in fluorescence images of the rectangle area in the left panel, taken at 110 K and 45 K. Right bottom: local magnetic field maps of the same area corresponding to the top images.

- 
- [1] Doherty, M. W. *et al.* The nitrogen-vacancy colour centre in diamond. *Physics Reports* **528**, 1–45 (2013).
  - [2] Mittiga, T. *et al.* Imaging the local charge environment of nitrogen-vacancy centers in diamond. *Physical review letters* **121**, 246402 (2018).
  - [3] Van Oort, E. & Glasbeek, M. Electric-field-induced modulation of spin echoes of nv centers in diamond. *Chemical Physics Letters* **168**, 529–532 (1990).
  - [4] Choi, J. *et al.* Depolarization dynamics in a strongly interacting solid-state spin ensemble. *Physical review letters* **118**, 093601 (2017).
  - [5] Ziffer, M. E. *et al.* Quantum noise spectroscopy of critical slowing down in an atomically thin magnet. *Under review at Science, preprint arXiv:2407.05614* (2024).
  - [6] Gullion, T., Baker, D. B. & Conradi, M. S. New, compensated carr-purcell sequences. *Journal of Magnetic Resonance (1969)* **89**, 479–484 (1990).
  - [7] Bauch, E. *et al.* Decoherence of ensembles of nitrogen-vacancy centers in diamond. *Physical Review B* **102**, 134210 (2020).
  - [8] Machado, F., Demler, E. A., Yao, N. Y. & Chatterjee, S. Quantum noise spectroscopy of dynamical critical phenomena. *Physical Review Letters* **131**, 070801 (2023).
  - [9] Zuo, Y. *et al.* Synthetic diamond for nitrogen vacancy sensor and its applicability. *Industries, Sumitomo Electric,(92)* **6** (2021).
  - [10] Ziegler, J. F., Ziegler, M. D. & Biersack, J. P. Srim—the stopping and range of ions in matter (2010). *Nuclear Instruments and Methods in Physics Research Section B: Beam Interactions with Materials and Atoms* **268**, 1818–1823 (2010).
  - [11] Hsieh, S. *et al.* Imaging stress and magnetism at high pressures using a nanoscale quantum sensor. *Science* **366**, 1349–1354 (2019).
  - [12] Wen, J. *et al.* Large bi-2212 single crystal growth by the floating-zone technique. *Journal of Crystal Growth* **310**, 1401–1404 (2008).
